# Supplementary material for: CMAL: A Novel Cross-Modal Associative Learning Framework for Vision-Language Pre-Training
Source: arXiv:2410.12595 source file (2024-10-16)
Supplement: Supplementary file 1 [file Appendices.tex]

% !TEX spellcheck = en_US
% !TeX root = main.tex

\clearpage

\section{Appendices}
\label{sec:appendix}
\subsection{Hyperparameters Setting}
\label{subsec: hypersetting}
The hyperparameters used for MMD dataset are shown in Table~\ref{tab:hyperparameters}.
\begin{table}[htbp]
	\centering
	\begin{tabular}{l|l}
		\hline
		\textbf{Hyperparameter Name} & \textbf{MMD}  \\
		\hline \hline
		Batch Size & 64     \\
		Epoches & 10,000 \\
		Text Embedding Size & 512   \\
		Image Embedding Size & 512    \\
		Transformer Embedding Size & 512 \\
		Learning Rate & 0.0001  \\
		Dropout Ratio & 0.15   \\
		Teacher Forcing Ratio & 0.9   \\
		Mask Length &  6 \\
		Mask Probability  &  0.15 \\
		Replace Probability & 0.15 \\
		Vocabulary Size & 26,422 \\
		\hline
	\end{tabular}%
	\caption{Hyperparameters we used for MMD.}
	\label{tab:hyperparameters}
	\vspace{-1em}
\end{table}%

\subsection{Description of Special Tokens}
The special tokens used in our experiments are shown in Table~\ref{tab:special_token}.

\subsection{Loss Function}
Our total loss function $\mathcal{L}_{Total}$ comprises three parts: UTS encoder loss $\mathcal{L}_{E}$, FAIR layer loss $\mathcal{L}_{F}$ and HTR decoder loss $\mathcal{L}_{D}$, which can be calculated as follows:
\begin{equation}
	\mathcal{L}_{Total}=\gamma_{E} \mathcal{L}_{E}+\gamma_{F} \mathcal{L}_{F}+\gamma_{D} \mathcal{L}_{D}
\end{equation}
where $\gamma_{E}$, $\gamma_{F}$ and $\gamma_{D}$ are hyperparameters, and are initialized equally, i.e., $0.33$, $0.33$ and $0.33$. Then, we tune them on the verification set to obtain a better weight setting of $0.30$, $0.35$ and $0.35$.

The UTS encoder loss $\mathcal{L}_{E}$ contains two parts: $\mathcal{L}_{\mathrm{MLM}}$ and $\mathcal{L}_{\mathrm{MPM}}$,
\begin{equation}
	\mathcal{L}_{E}=\mathcal{L}_{\mathrm{MLM}}+\mathcal{L}_{\mathrm{MPM}}
\end{equation}
the FAIR layer loss contains three parts: $\mathcal{L}_{\mathrm{ITM}}$, $\mathcal{L}_{\mathrm{WPA}}$ and $\mathcal{L}_{\mathrm{IC}}$:
\begin{equation}
	\mathcal{L}_{F}=\mathcal{L}_{\mathrm{ITM}}+\mathcal{L}_{\mathrm{WPA}}+\mathcal{L}_{\mathrm{IC}}
\end{equation}
and the HTR decoder loss is divided into two types: the textual decoding loss $\mathcal{L}_{\mathrm{TXT}}$ for text task and image recommend loss $\mathcal{L}_{\mathrm{IMG}}$ for image task, which is consistent with previous work~\cite{DBLP:conf/mm/NieWHWT19}.  
\begin{equation}
	\mathcal{L}_{D}=\mathcal{L}_{\mathrm{TXT}}+\mathcal{L}_{\mathrm{IMG}}
\end{equation}

\begin{table}[]
	\centering
	\begin{tabular}{l|l}
		\hline
		\textbf{Token}      & \textbf{Description}                    \\ \hline \hline
		{[}CLS{]}  & Utterances classfication token \\ \hline
		{[}TXT{]}  & Text token                     \\ \hline
		{[}IMG{]}  & Image token                    \\ \hline
		{[}KNG{]}  & Knowledge token                \\ \hline
		{[}MASK{]} & Mask token                     \\ \hline
		{[}URL{]} & Image link token  \\ \hline
		{[}PAD{]} & Padding token  \\ \hline
		{[}UNK{]} & Unknown token  \\ \hline
	\end{tabular}
	\caption{Description of special tokens in our experiments.}
	\label{tab:special_token}
	\vspace{-1em}
\end{table}

\subsection{Dateset Statistics}
\label{sec: statistics}
A detailed statistics of the MMD dataset is presented in Table~\ref{tab: detail_statistics}.
\begin{table}[]
	\centering
	\begin{tabular}{l|c|c|c}
		\hline
		\textbf{Dataset Statistics}                       & \textbf{Train}   & \textbf{Valid}  & \textbf{Test}   \\ \hline \hline
		Dialogs             & 105,439 & 22,595 & 22,595 \\ \hline
		Proportion           & 70\%    & 15\%   & 15\%   \\ \hline
		Questions      & 2M      & 446K   & 445K   \\  \hline
		Image Responses         & 904K    & 194K   & 193K   \\  \hline
		Text Responses          & 1.54M   & 331K   & 330K   \\  \hline
		Avg. Utterances            & 40      & 40     & 40     \\  \hline
		Avg. Pos. Images  & 4       & 4      & 4      \\  \hline
		Avg. Neg. Images & 4       & 4      & 4      \\  \hline
		Avg. Words in Question       & 12      & 12     & 12     \\  \hline
		Avg. Words in Response            & 14      & 14     & 14     \\ \hline
	\end{tabular}
	\caption{Detailed statistics of the MMD dataset.}
	\label{tab: detail_statistics}
	\vspace{-1em}
\end{table}

\subsection{Error Analysis}
To better understand the limitations of our model, we conduct an error analysis on UniTranSeR. We randomly select $100$ responses generated by UniTranSeR that achieve low human evaluation scores in the test set of MMD. We report several reasons for the low  scores, which can roughly be classified into four categories. (1) KB information in the generated responses is incorrect ($38\%$), especially when the corresponding equipped knowledge base is large and complex. (2) The sentence structure of the generated responses is incorrect and there are serious grammatical and semantic errors ($24\%$). (3) The model makes incomplete response when there are multiple intentions contained in users' utterances ($21\%$). 
(4) The model selects incorrect product images since different products have similar attributes ($17\%$).
